# Supplementary material for: FloydNet: A Learning Paradigm for Global Relational Reasoning
Source: arXiv:2601.19094 source file (2026-09-01)
Supplement: Supplementary file 1 [file appendix_lrgb_data_size.tex]

\begin{table*}[h!]
\centering
\caption{Statistics of the five proposed LRGB datasets.}
\label{tab:lrgb_datasize}

 % 行距
\setlength{\tabcolsep}{10pt}      % 列间距

\begin{tabular}{lrrrr}
\toprule
\textbf{Dataset} & \textbf{Total Graphs} & \textbf{Avg Nodes} & \textbf{Avg Edges} & \textbf{Mean Deg.} \\
\midrule
PascalVOC-SP    & 11,355  & 479.40  & 2,710.48 & 5.65 \\
COCO-SP         & 123,286 & 476.88  & 2,693.67 & 5.65 \\
PCQM-Contact    & 529,434 & 30.14   & 61.09    & 2.03 \\
Peptides-func   & 15,535  & 150.94  & 307.30   & 2.04 \\
Peptides-struct & 15,535  & 150.94  & 307.30   & 2.04 \\
\bottomrule
\end{tabular}
\end{table*}
